# Supplementary material for: Correlation between ferroelectricity and torsional motion of acetyl groups in tris(4-acetylphenyl)amine observed by muon spin relaxation
Source: arXiv:2501.16685 source file (2025-01-28)
Supplement: Supplementary file 1 [file SM-v2.1.pdf]

# Supplementary Material

for

# Correlation between ferroelectricity and torsional motion of acetyl group in tris(4-acetylphenyl)amine observed by muon spin relaxation

by

J. G. Nakamura[1], M. Hiraishi[1,2], H. Okabe[1,3], A. Koda1[4], R. Kumai[5,4], F. L. Pratt[6], and R. Kadono[1]

[1]*Muon Science Laboratory, Institute of Materials Structure Science, High Energy Accelerator Research Organization (IMSS, KEK), Oho, Tsukuba, Ibaraki 305-0801, Japan*
[2]*Graduate School of Science and Engineering, Ibaraki University, Bunkyo, Mito, Ibaraki 310-8512, Japan*
[3]*Institute for Materials Research, Tohoku University (IMR), Katahira, Aoba-ku, Sendai 980-8577, Japan*
[4]*Graduate Institute for Advanced Studies, SOKENDAI*
[5]*Photon Factory, Institute of Materials Structure Science, High Energy Accelerator Research Organization (IMSS, KEK), Oho, Tsukuba, Ibaraki 305-0801, Japan*
[6]*ISIS Facility, STFC Rutherford Appleton Laboratory, Chilton, Oxfordshire OX11 0QX, United Kingdom*

## I. Summary of the DFT calculations

Single molecule calculations were made of the relaxed structures and hyperfine coupling tensors for muoniated radicals formed by addition of muonium to double bonds in the structure. The numbering of the sites is shown in Fig.S1. The Gaussian 16 package running on the STFC SCARF Compute Cluster was used for the calculations, supervised by the CalcALC program. The starting point is the structure of a single molecule extracted from the full crystallographic structure. An efficient computation method for the muoniated states was employed that starts by adding muonium to a selected site and obtaining the relaxed structure using the PM7 semi-empirical Hartree-Fock method, which is based on machine-learning principles. The electronic properties are then obtained using DFT with the hybrid B3LYP density functional along with the cc-pVDZ basis set. The obtained energies and hyperfine tensors are listed in Table S1. Where two hyperfine tensors are given, they refer to addition above and below the plane of the phenylene ring. A quantum correction factor of 1.23 was applied to the A values of the C addition sites, this factor was obtained by calibration of the DFT calculation method against solid benzene. No thermal correction factor was applied here, so the calculations are for T = 0 K. Addition to the central N is expected to be at much higher energy than the sites listed in Table 1 and we confirmed this by calculation, finding that it is 2.1 eV higher than the O site. Various factors such as thermal correction and solid-state interactions are not included with this type of calculation, but the ordering of the energies and the ratios of muon hyperfine parameters between different sites are expected to be well reproduced by this approach and the absolute magnitudes of the HFC can be corrected by a simple scaling factor that is close to one.

Fig.S1 Site numbering of TAPA:
gray = C, white= H, red = O, blue = N

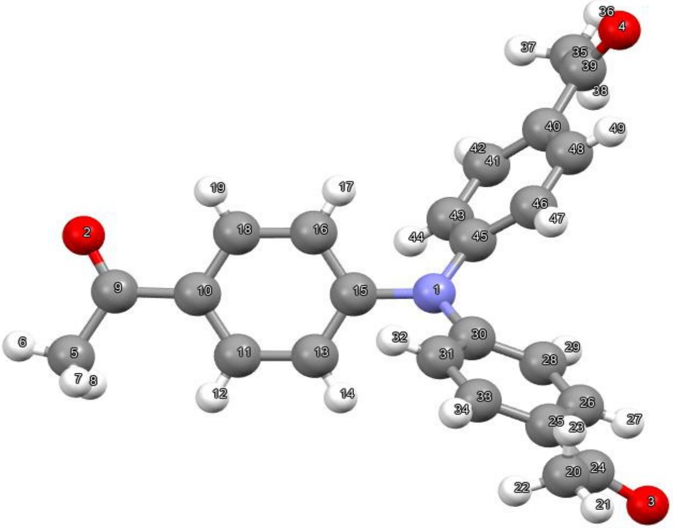

Table S1 Hyperfine coupling tensors of muoniated radicals associated with atoms on TAPA molecule (where the figures are those without the factor $2\pi$). The last two columns show the strongest coupled H sites with their corresponding NHF values $A_H$.

| Addition Site | Energy (eV) | Hyperfine coupling tensor ($A$, $D_1$, $D_2$) in MHz | | Strongest NHF coupled H sites | $A_H$ (MHz) |
|---|---|---|---|---|---|
| O2 | −0.310 | (−32.2, 52.8, 11.5) | | 7, 8 | 55 |
| C9 | 0.671 | (914.2, 36, 24.9) | | 6 | 3 |
| C10 | 0.331 | (358.8, 9.3, 7.9) | (358.8, 9.3, 7.9) | 12, 19 | 22 |
| C11 | 0.072 | (515.1, −12.0, 11.6) | (490.1, 12.4, 12.0) | 12 | 110 |
| C13 | 0.183 | (460.7, 11.2, 11.2) | (480.4, −10.5, 8.1) | 14 | 123 |
| C15 | 0.487 | (527.2, 7.7, 5.4) | (530.5, 7.6, 5.4) | 14, 17 | -24 |
| C16 | 0.163 | (485.4, −10.6, 8.5) | (472.2, −11.4, 11.4) | 17 | 121 |
| C18 | 0 | (482.6, −12.8, 11.1) | (536.0, −12.8, 10.8) | 19 | 137 |

Fig. S2 Examples of muoniated structures of TAPA molecule with Mu sites shown by pink balls. The O2 and C9 sites are associated with the acetyl groups, and others are with phenyl groups.

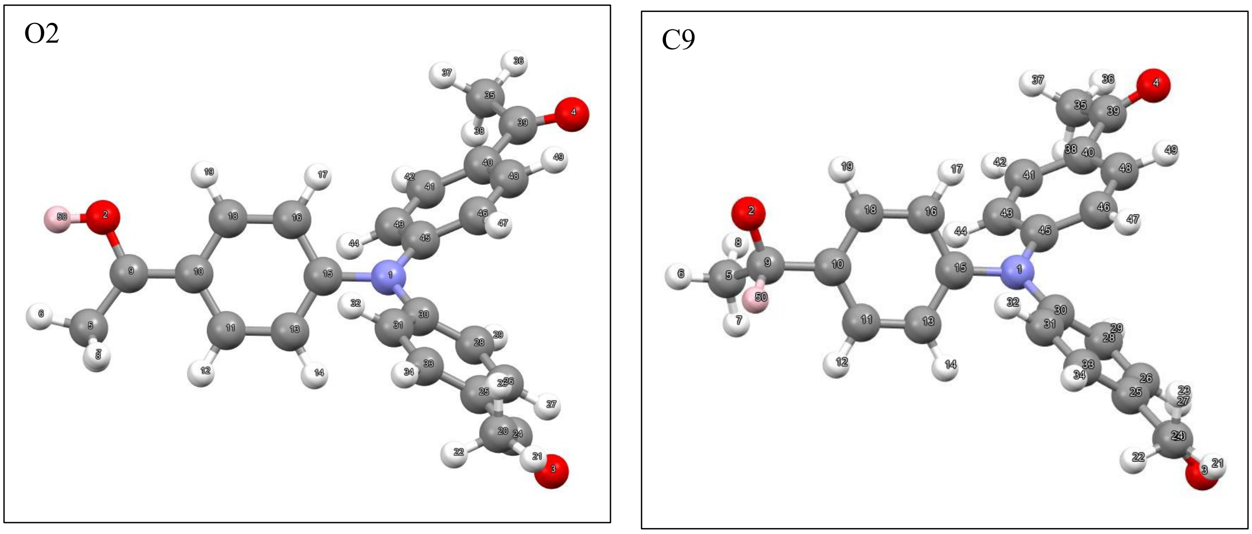

C11

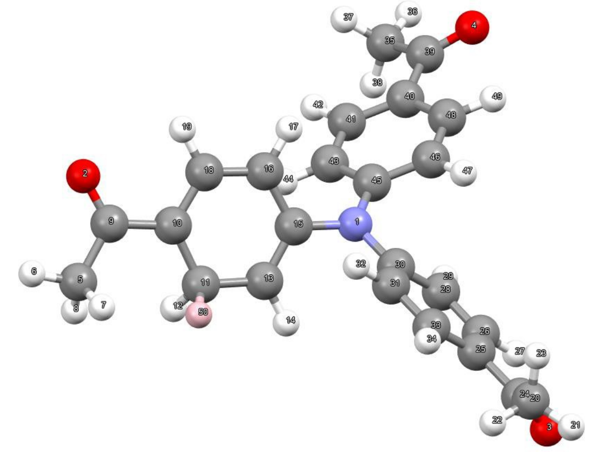

C13

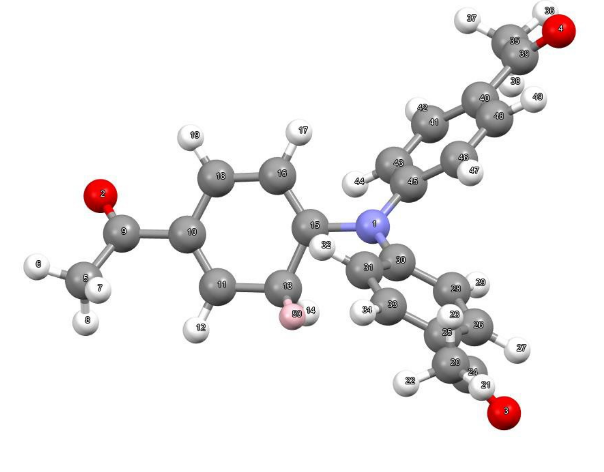

C10

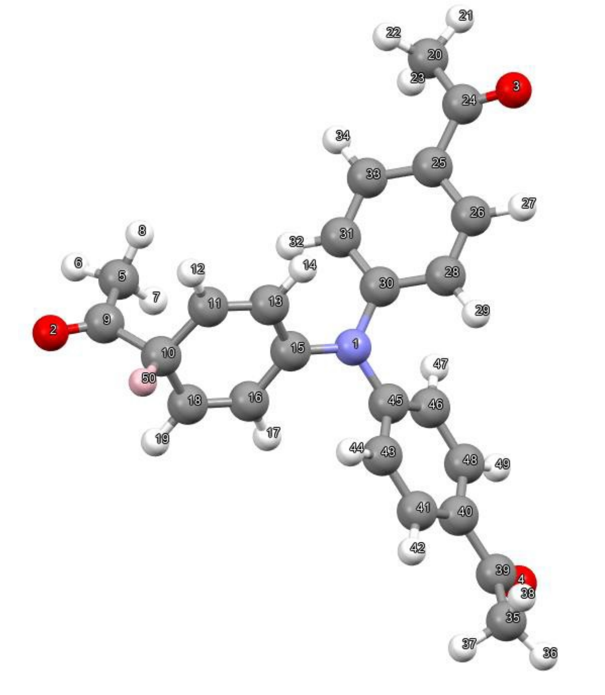

C15

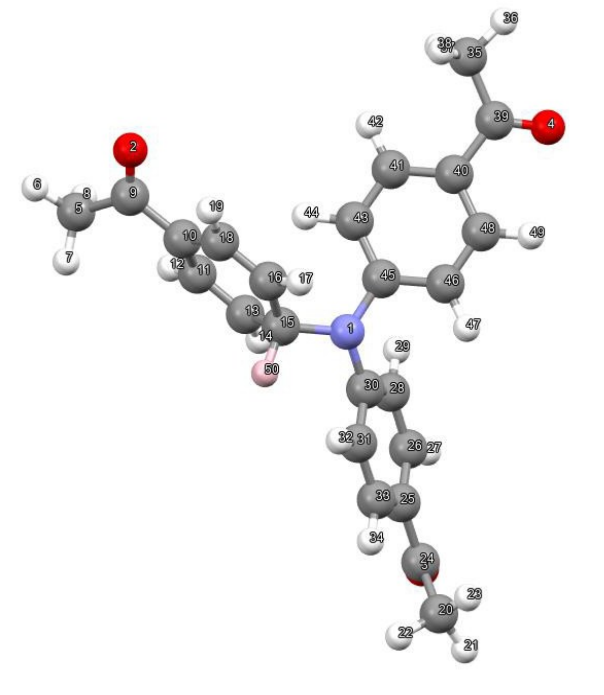

C16

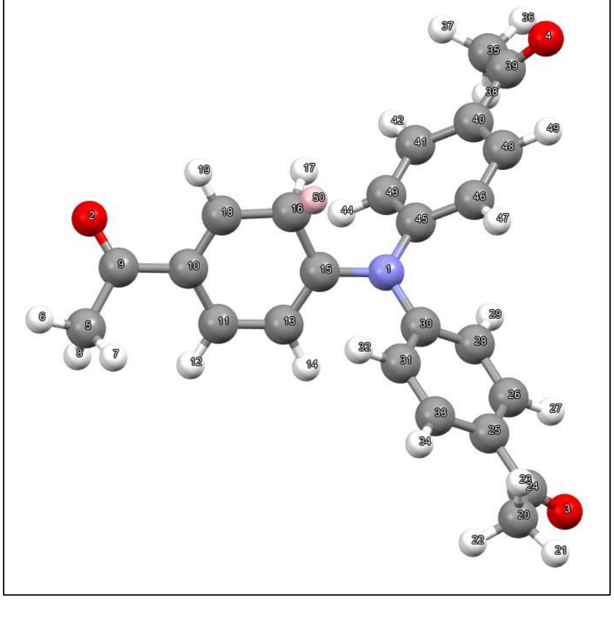

C18

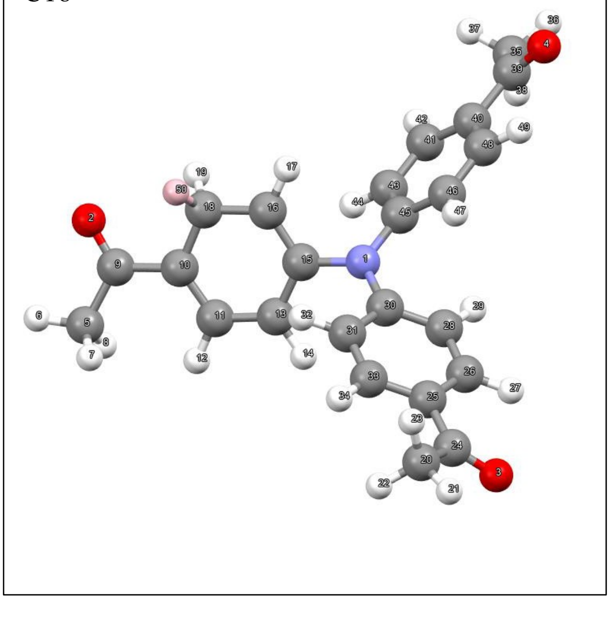

## II. Analytical approximation of LF-repolarization curves predicted by CalcALC

The LF-dependence of the initial muon polarization calculated by the CalcALC program was fitted by the following form:

$$P(B) = m_1 + m_2 \frac{\frac{1}{2}\left[\frac{m_3+x_n^2}{1+x_n^2}\right]+x_p^2}{1+x_p^2},\ x_p = \frac{2\gamma_{av}B}{\omega_0},\ x_n = \frac{\gamma_{av}B}{\Delta_n}$$

$\gamma_{av} = (\gamma_e + \gamma_\mu)/2,\ \omega_0$ : HF, $\Delta_n$ : NHF

where $m_1$ and $m_2$ are parameters for fits using the least-square method. The results of fits are shown below for Mu radicals associated with C11, C9, and O2.

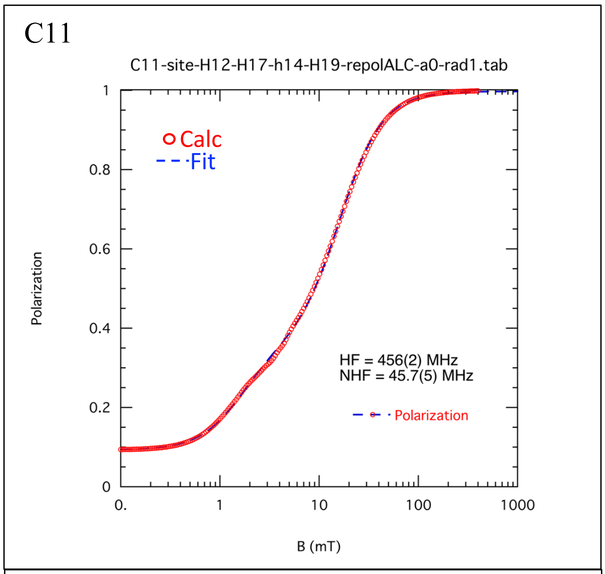


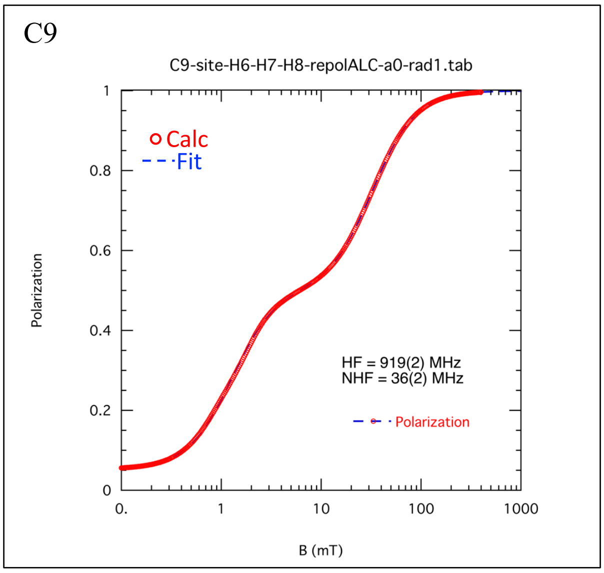


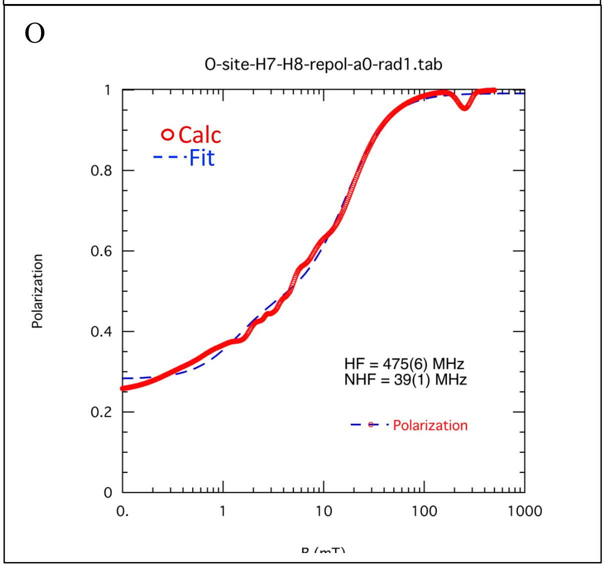


Fig. S3 Results of curve fits for $P(B)$ vs. $B$ for C11, C9, and O2 radicals, where the obtained parameters are listed in Table S2.

Table S2 Parameters (divided by $2\pi$) of the polarization function $P(B)$ approximating the $B$ dependence given numerically by CalcALC .

| Mu site | HF (MHz) | NHF (MHz) |
|---|---|---|
| C11 | 456(2) | 45.7(5) |
| C9 | 919(2) | 36(2) |
| O | 475(6) | 39(1) |

The analytical approximation works well for each Mu radical state, yielding reasonable HF parameters and (mean) NHF parameters. The relative weight between C11 and C9 can be discerned by $P(B)$ around 10-200 mT.

III. Information on curve fit parameters omitted in the main text.

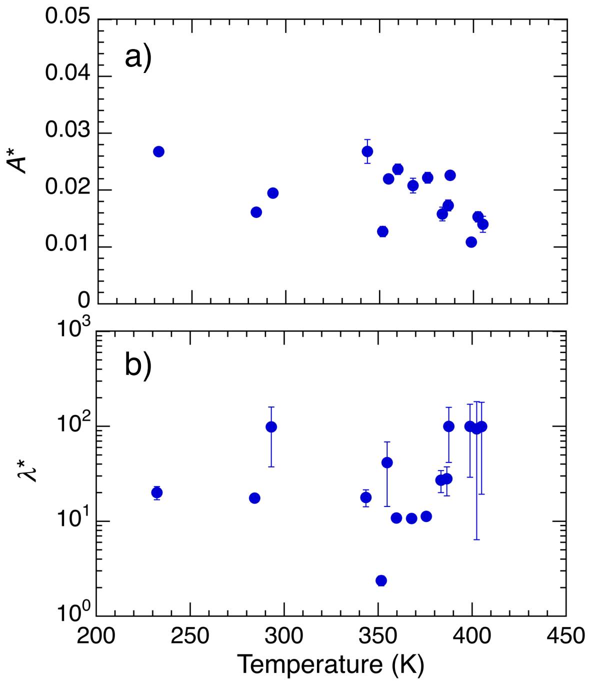


Fig.S4 Temperature dependence of the initial asymmetry $A^*$ and the relaxation rate $\lambda^*$ of the fast-damping paramagnetic component in TAPA. The scattering in $\lambda^*$ is due to artifacts associated with the difficulty of deriving the large relaxation rates (>10 MHz) exhibited by signals with small asymmetry ($A^*$~0.02) in the curve fit, which is due to the insufficient statistical precision in the corresponding time region (<0.1μs).

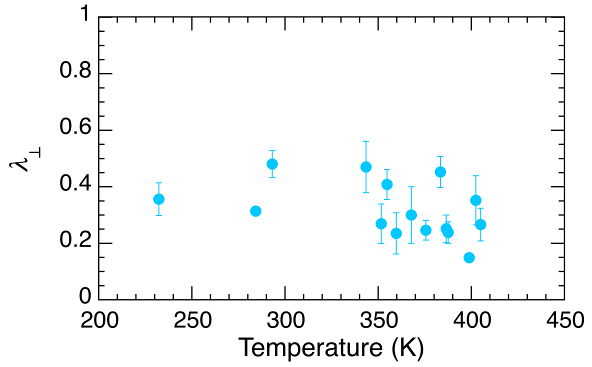


Fig.S5 Temperature dependence of the relaxation rate $\lambda_\perp$ of the slowly damping diamagnetic component in TAPA.

IV. Crystallography

The X-ray diffraction data for TAPA at high temperature were collected with a Rigaku DSC imaging plate system by using Si-double-crystal monochromatized synchrotron radiation (λ = 1.00 Å) installed in the beam line BL-8A of Photon Factory (PF), High-Energy Accelerator Research Organization (KEK). The monochromatized beam is focused using a bent cylindrical mirror made of Si crystal coated with Rh, with a focused beam size of 0.3 (vertical) × 0.7 (horizontal) mm. The crystal attached on a glass fiber was heated by flowing nitrogen gas. The diffraction measurement was performed at $T$ = 430 K. The Rapid-AUTO program of Rigaku Corp. was employed for two-dimensional image processing. The SHELX programs [G. M. Sheldrick, Crystal structure refinement with SHELXL. *Acta Cryst.* **C71**, 3-8 (2015)] were employed for the refinement of the structures. The final refinements of non-hydrogen atoms were done with anisotropic thermal factors.

Crystallographic data collection and structural refinement information for TAPA at high temperature was summarized in Table S3.

Table S3. Crystal data of TAPA at 430 K.

| | |
|---|---|
| Radiation | Synchrotron ($\lambda$ = 1.00 Å) |
| Formula | $C_{24}H_{21}NO_3$ |
| Formula weight | 371.43 |
| Crystal system | orthorhombic |
| Space group | *Pbcn* (No.60) |
| Crystal color | Colorless |
| Crystal description | block |
| $a$ [Å] | 8.7830(2) |
| $b$ [Å] | 12.0314(3) |
| $c$ [Å] | 19.2492(4) |
| $V$ [Å$^3$] | 2034.10(8) |
| $Z$ | 4 |
| $d_{calcd}$ [g cm$^{-3}$] | 1.213 |
| $R_{int}$ | 0.0241 |
| $2\theta_{max}$ [°] | 74 |
| reflections | 1481 |
| parameters | 174 |
| $R_1$ ($I > 2\sigma(I)$) | 0.0760 |
| $wR_2$ (all data) | 0.2592 |
| Goodness-of-fit | 1.071 |
| Temperature [K] | 430(1) |

With increasing temperature, the lattice parameters show large change at the Curie temperature and the $hk0$ ($k$ = 2n) reflections, which can be observed in the space group ($Pna2_1$) at room temperature disappears above transition temperature (Fig. S6). This indicates a structural transition to the symmetric-centered space group, *Pnab*. The structure at high temperature was refined as *Pbcn* by the following lattice transformation.

$$\begin{pmatrix} a_{HT} \\ b_{HT} \\ c_{HT} \end{pmatrix} = \begin{pmatrix} 0 & 0 & 1 \\ 0 & -1 & 0 \\ 1 & 0 & 0 \end{pmatrix} \begin{pmatrix} a_{RT} \\ b_{RT} \\ c_{RT} \end{pmatrix}$$

Temperature dependence of the lattice parameters including above and below Curie temperature (Fig. 4(d)), was obtained by cell refinement using three oscillation photographs at each temperature.

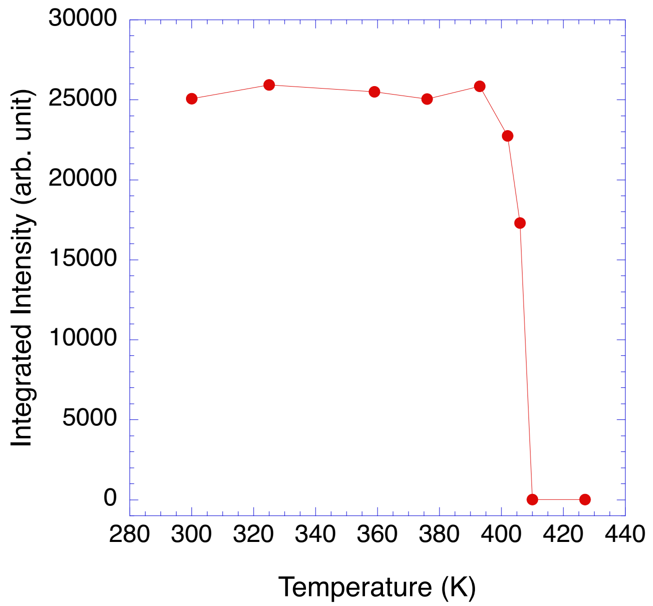


Fig. S6. Temperature dependence of integrated intensity of 710 reflection (*Pnab* setting).

Temperature dependence of the atomic displacement parameters (Fig. 4(e)) was determined by structural refinement at each temperature between 200 K and 400 K using synchrotron radiation (λ = 1.00 Å) in the same way as for the structural analysis of high temperature phase at beamline BL-8A of Photon Factory. The structure refinement information is summarized in Table S4.

Table S4. Crystal data of TAPA between 200 K and 400 K.

| Temperature [K] | 200 | 250 | 300 | 320 | 340 |
|---|---|---|---|---|---|
| Radiation | | | Synchrotron (λ = 1.00 Å) | | |
| Formula | | | $C_{24}H_{21}NO_3$ | | |
| Formula weight | | | 371.43 | | |
| Crystal system | | | orthorhombic | | |
| Space group | | | $Pna2_1$ (No. 33) | | |
| $a$ [Å] | 18.5907(7) | 18.6386(7) | 18.6935(7) | 18.7163(7) | 18.7408(7) |
| $b$ [Å] | 11.8663(2) | 11.8845(2) | 11.9044(2) | 11.9126(2) | 11.9200(2) |
| $c$ [Å] | 8.6513(2) | 8.6886(2) | 8.7313(2) | 8.7500(2) | 8.7699(2) |
| $V$ [Å$^3$] | 1908.50(9) | 1924.62(8) | 1943.02(9) | 1950.90(9 | 1959.11(9) |
| $Z$ | | | 4 | | |
| $d_{calcd}$ [g cm$^{-3}$] | 1.293 | 1.282 | 1.27 | 1.265 | 1.259 |
| $R_{int}$ | 0.0133 | 0.0234 | 0.0145 | 0.0178 | 0.021 |
| $2\theta_{max}$ [°] | 130 | 130 | 112 | 100 | 100 |
| reflections | 7048 | 7094 | 5885 | 4927 | 4930 |
| parameters | 257 | 257 | 257 | 257 | 257 |

| | | | | | |
|---|---|---|---|---|---|
| $R_1$ ($I > 2\sigma(I)$) | 0.0407 | 0.0517 | 0.0437 | 0.0408 | 0.0481 |
| $wR_2$ (all data) | 0.1068 | 0.1549 | 0.1266 | 0.1214 | 0.1548 |
| Goodness-of-fit | 0.977 | 0.96 | 0.919 | 0.979 | 0.985 |

| Temperature [K] | 360 | 370 | 380 | 390 | 400 |
|---|---|---|---|---|---|
| Radiation | | | Synchrotron (λ = 1.00 Å ) | | |
| Formula | | | $C_{24}H_{21}NO_3$ | | |
| Formula weight | | | 371.43 | | |
| Crystal system | | | orthorhombic | | |
| Space group | | | $Pna2_1$ (No. 33) | | |
| $a$ [Å] | 18.7673(7) | 18.7825(7) | 18.8009(7) | 18.8209(7) | 18.8449(7) |
| $b$ [Å] | 11.9289(2) | 11.9336(2) | 11.9398(2) | 11.9461(2) | 11.9537(2) |
| $c$ [Å] | 8.7905(2) | 8.8010(2) | 8.8123(2) | 8.8232(2) | 8.8338(2) |
| $V$ [Å$^3$] | 1967.96(9) | 1972.68(9) | 1978.18(9) | 1983.78(9) | 1989.96(9) |
| $Z$ | | | 4 | | |
| $d_{calcd}$ [g cm$^{-3}$] | 1.254 | 1.251 | 1.247 | 1.244 | 1.24 |
| $R_{int}$ | 0.0158 | 0.0187 | 0.013 | 0.0155 | 0.017 |
| $2\theta_{max}$ [°] | 94 | 91 | 91 | 91 | 81 |
| reflections | 4495 | 4221 | 4249 | 4258 | 3457 |
| parameters | 257 | 257 | 257 | 257 | 257 |
| $R_1$ ($I > 2\sigma(I)$) | 0.0393 | 0.0456 | 0.0425 | 0.0403 | 0.0392 |
| $wR_2$ (all data) | 0.1196 | 0.1517 | 0.1401 | 0.1301 | 0.121 |
| Goodness-of-fit | 0.973 | 1.052 | 1.059 | 0.999 | 1.028 |
